# Supplementary material for: Generating Optimal Grasps Under A Stress-Minimizing Metric
Source: arXiv:1907.08749 source file (2019-07-20)
Supplement: Supplementary file 1 [file appendix_A2.tex]

\subsection{Another Derivation of BIE}
We can also derive BIE by expanding operator $\LL$ and use the vector-valued divergence theorem:
\begin{align*}
 \int_\Omega \vv^T\nabla\nabla\cdot\uu d\xx 
=&\int_\Omega \nabla\cdot(\vv\nabla\cdot\uu) d\xx - \int_\Omega \nabla\cdot\uu\nabla\cdot\vv d\xx   \\
=&\int_{\partial\Omega} \vv^T\nabla\cdot\uu\nn d\pxx - \E{Sym}(\uu,\vv)    \\
 \int_\Omega \vv^T\Delta\uu d\xx    
=&\int_\Omega \nabla\cdot(\nabla\uu^T\vv) d\xx - \int_\Omega \tr{\nabla\vv^T\nabla\uu} d\xx   \\
=&\int_{\partial\Omega} \vv^T\nabla\uu\nn d\pxx - \E{Sym}(\uu,\vv).
\end{align*}
We also need to use the following identity:
\begin{align*}
\int_{\partial\Omega} \vv^T\nabla\cdot\uu\nn d\pxx = \int_{\partial\Omega} \vv^T\nabla\uu^T\nn d\pxx + \E{Sym}(\uu,\vv).
\end{align*}
Combining these two equations and we get:
\begin{align*}
 &\int_\Omega \vv^T\LL[\uu] d\xx  \\
=&-\int_{\partial\Omega} \vv^T\left[(\mu+\lambda)\nabla\cdot\uu\nn+\mu\nabla\uu\nn\right] d\pxx + \E{Sym}(\uu,\vv) \\
=&-\int_{\partial\Omega} \vv^T\left[\lambda\nabla\cdot\uu\nn+\mu\nabla\uu^T\nn+\mu\nabla\uu\nn\right] d\pxx + \E{Sym}(\uu,\vv)    \\
=&-\int_{\partial\Omega} \vv^T\NN[\uu] d\pxx + \E{Sym}(\uu,\vv).
\end{align*}
